# Supplementary material for: A Non-Convex Optimization Technique for Sparse Blind Deconvolution -- Initialization Aspects and Error Reduction Properties
Source: arXiv:1708.07370 source file (2017-10-11)
Supplement: Supplementary file 1 [file ex_supplement.tex]

\documentclass[final,supplement]{siamart1116}
% SIAM Shared Information Template
% This is information that is shared between the main document and any
% supplement. If no supplement is required, then this information can
% be included directly in the main document.

% Packages and macros go here
\usepackage{lipsum}
\usepackage{amsfonts}
\usepackage{graphicx}
\usepackage{epstopdf}
\usepackage{algorithmic}
\ifpdf
  \DeclareGraphicsExtensions{.eps,.pdf,.png,.jpg}
\else
  \DeclareGraphicsExtensions{.eps}
\fi

%strongly recommended
\numberwithin{theorem}{section}

% Declare title and authors, without \thanks
\newcommand{\TheTitle}{An Alternating Minimization Strategy for Sparse Blind Deconvolution $-$ Convergence Analysis and Concentration Inequalities}
\newcommand{\PageTitle}{1-D Sparse Blind Deconvolution}
\newcommand{\TheAuthors}{Aniruddha Adiga and Chandra Sekhar Seelamantula}

% Sets running headers as well as PDF title and authors
\headers{\PageTitle}{\TheAuthors}

% Title. If the supplement option is on, then "Supplementary Material"
% is automatically inserted before the title.
\title{{\TheTitle}}
%\thanks{Submitted to the editors DATE.\funding{Science and Engineering Research Board, Government of India.}}}

% Authors: full names plus addresses.
\author{
  Aniruddha Adiga$^\dagger$ \and
  Chandra Sekhar Seelamantula\thanks{Department of Electrical Engineering, Indian Institute of Science, Bangalore, India (\email{{aniruddha, chandra.sekhar}@ee.iisc.ernet.in}).}
}

\usepackage{amsopn}

%%% Local Variables: 
%%% mode:latex
%%% TeX-master: "ex_article"
%%% End: 

\externaldocument{ex_article}
% Optional PDF information
\ifpdf
\hypersetup{
  pdftitle={Supplementary Materials: \TheTitle},
  pdfauthor={\TheAuthors}
}
\fi
\begin{document}

\maketitle

\section{A detailed example}

Here we include some equations and theorem-like environments to show
how these are labeled in a supplement and can be referenced from the
main text.
Consider the following equation:
\begin{equation}
  \label{eq:suppa}
  a^2 + b^2 = c^2.
\end{equation}
You can also reference equations such as \cref{eq:matrices,eq:bb} 
from the main article in this supplement.

\lipsum[100-101]

\begin{theorem}
  An example theorem.
\end{theorem}

\lipsum[102]
 
\begin{lemma}
  An example lemma.
\end{lemma}

\lipsum[103-105]

Here is an example citation: \cite{KoMa14}.

\section[Proof of Thm]{Proof of \cref{thm:bigthm}}
\label{sec:proof}

\lipsum[106-114]

\section{Additional experimental results}
\Cref{tab:foo} shows additional
supporting evidence. 

\begin{table}[htbp]
  \caption{Example table}
  \label{tab:foo}
  \centering
  \begin{tabular}{|c|c|c|} \hline
   Species & \bf Mean & \bf Std.~Dev. \\ \hline
    1 & 3.4 & 1.2 \\
    2 & 5.4 & 0.6 \\ \hline
  \end{tabular}
\end{table}

\bibliographystyle{siamplain}
\bibliography{references}

\end{document}
